# Supplementary material for: FedNew: A Communication-Efficient and Privacy-Preserving Newton-Type Method for Federated Learning
Source: arXiv:2206.08829 source file (2022-06-17)
Supplement: Supplementary file 1 [file appendix.tex]

\onecolumn
\appendix
\section*{Appendices}

\if0

\section{Additional Experiments}\label{add_experiments}
In this section, we present more experiments for the a1a dataset. In Fig. \ref{fig3}, we present the optimality gap as a function of the number of communication rounds (on the left) and the communication bits per node (on the right).
\begin{figure*}[h]
\centering
\begin{subfigure}{.48\textwidth}
  \centering
\includegraphics[scale=0.50]{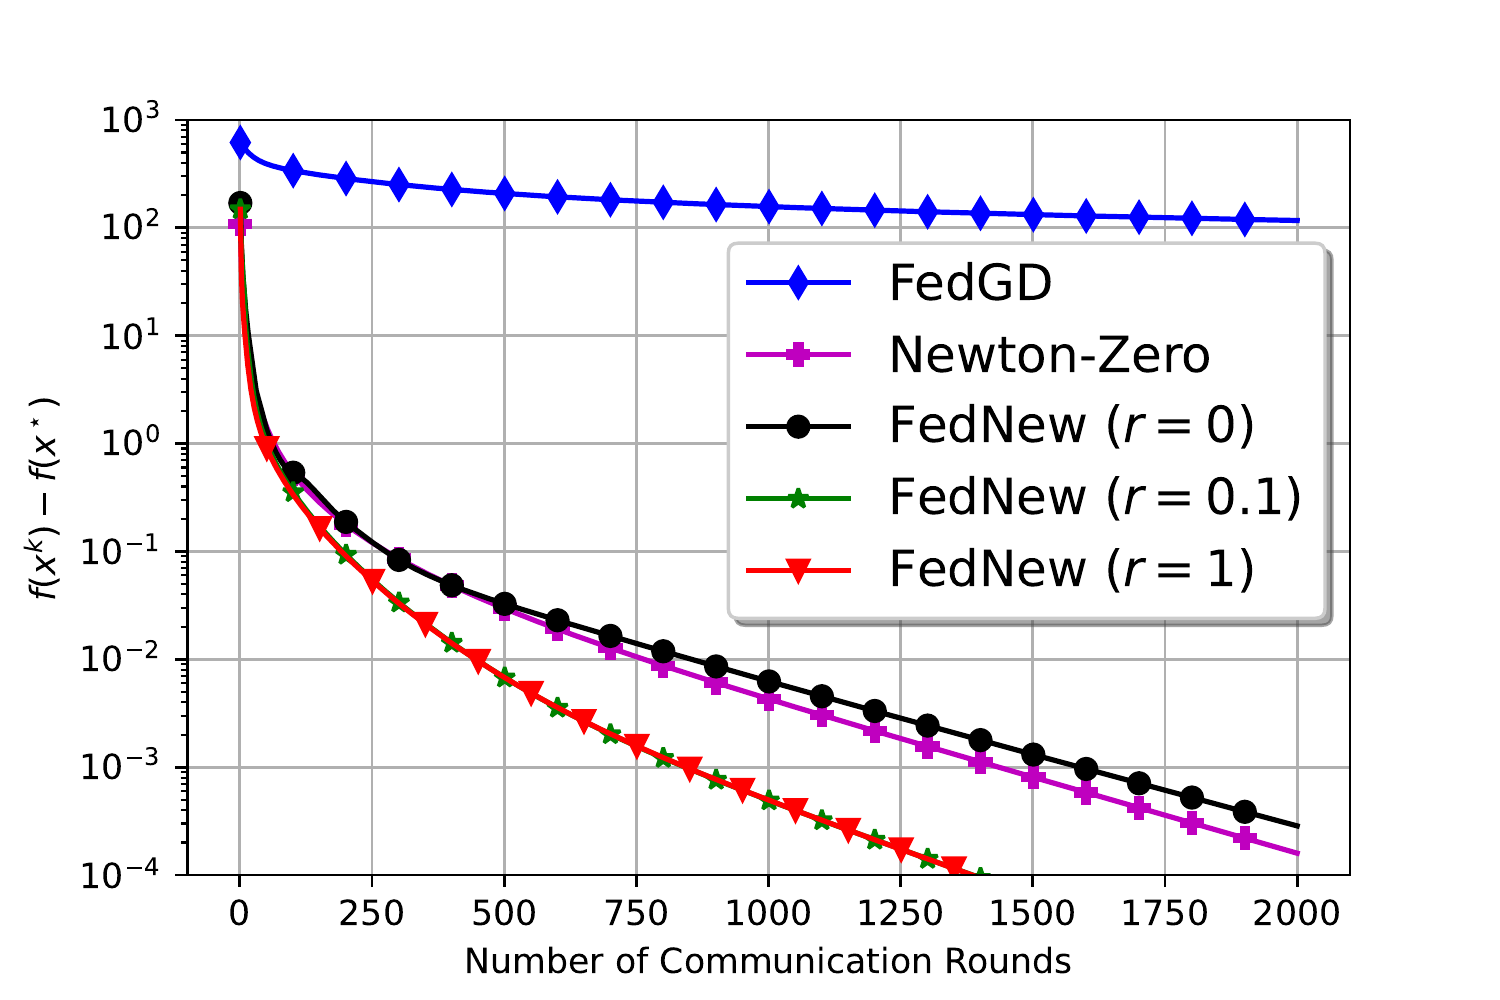} 
  %\caption{Dataset: a9a}
\end{subfigure}
\begin{subfigure}{.48\textwidth}
  \centering
\includegraphics[scale=0.50]{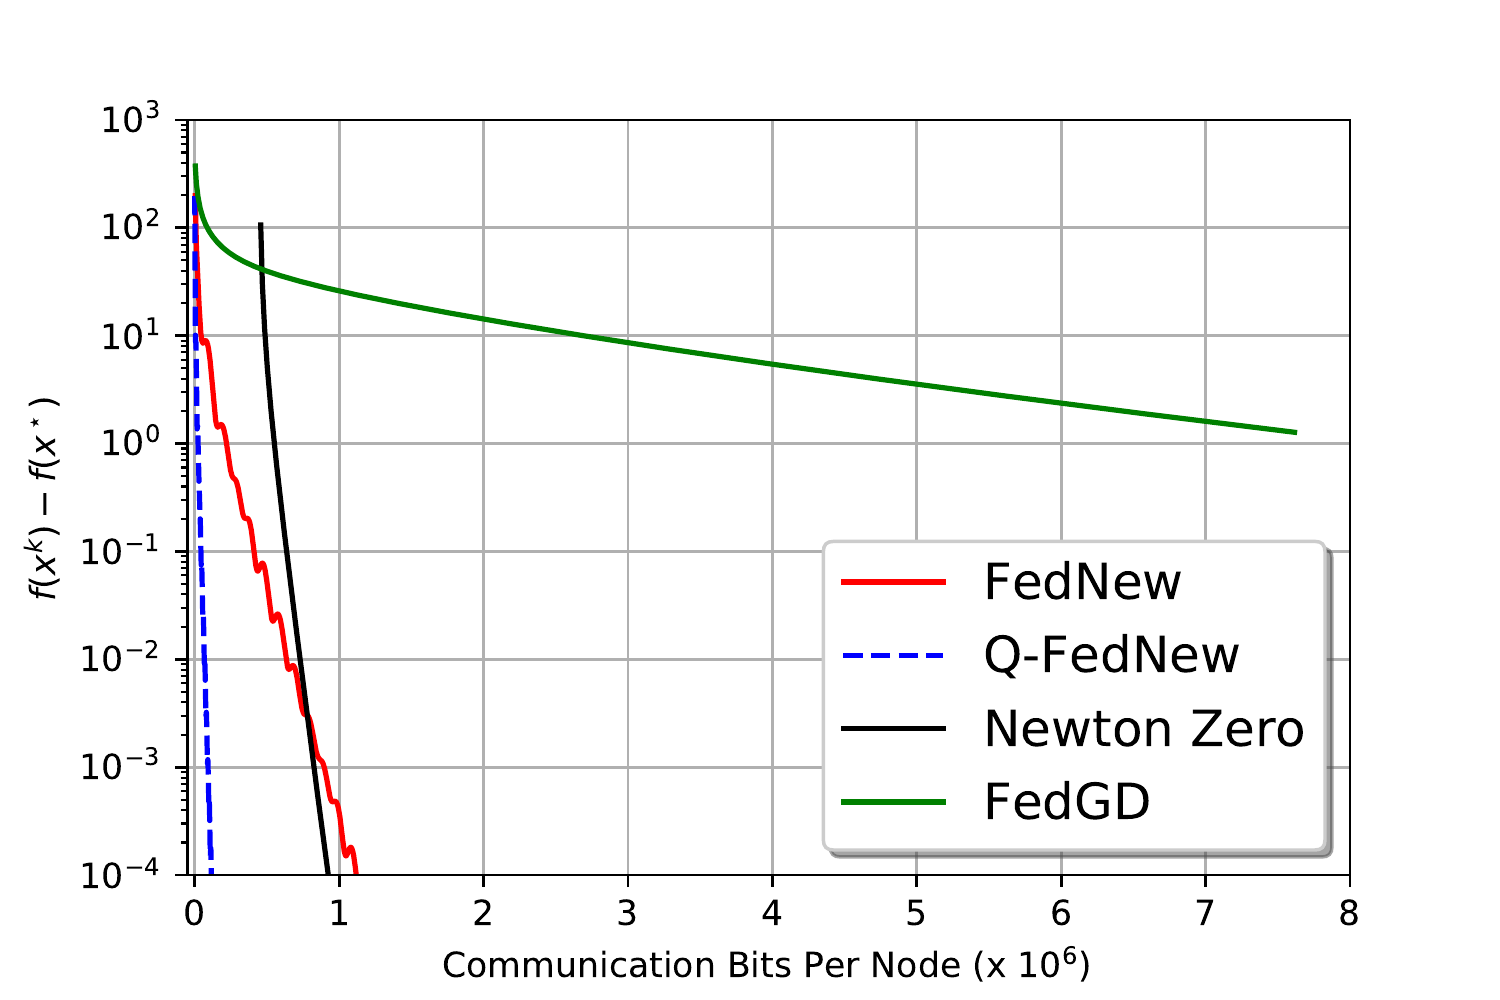} 
 % \caption{Dataset: w7a}
\end{subfigure}
\caption{Optimality gap of {\ours} and Q-{\ours} compared to Newton Zero in terms of number of communication rounds and communication bits per client for a9a dataset.}
\label{fig3}
\end{figure*}
\fi
\section{Proof of Lemma \ref{lemma_1}}\label{proof_lemma_1}
At iteration $k$, and given $x^k$, we run the one step ADMM to evaluate the direction $y_i^k$ at each client $i$. From the first order optimality condition of the problem in \eqref{updateLocal}, we can write
\begin{align}\label{feasi0}
 (H_i^k+\alpha I) y_i^k-g_i^k + \lambda_i^{k-1} + \rho (y_i^k - y^{k-1}) =0.
\end{align}
We add and subtract $y^{k}$ in the left hand side in the above expression and utilize the dual udpate  $\lambda_{i}^{k}=\lambda_{i}^{k-1}+ \rho (y_{i}^{k} - y^{k})$ (cf. \eqref{updateDual})  in \eqref{feasi0} to get 
\begin{align}\label{eqo10}
(H_i^k+\alpha I) y_i^k-g_i^k + \lambda_i^k + \rho (y^{k} - y^{k-1})=0.
\end{align}
Let $s^k$ be the dual residual at iteration $k$ defined as 
\begin{equation}\label{dualResidualEq}
s^k=\rho(y^{k}-y^{k-1})
\end{equation}
Therefore, \eqref{eqo10} can be re-written as
\begin{align}\label{eqo20}
(H_i^k+\alpha I) y_i^k-g_i^k + \lambda_i^k + s^k = 0.
\end{align}
Re-arranging the terms, we get
\begin{align}\label{eqo200}
\lambda_i^k + s^k = g_i^k -(H_i^k+\alpha I) y_i^k.
\end{align}
Subtracting ${\lambda_i^\star}^k$ from both sides and using \eqref{dual_feasibility}, we obtain
\begin{align}\label{}
\lambda_i^k + s^k-{\lambda_i^\star}^k = (H_i^k+\alpha I)({y_i^\star}^k-y_i^k)
\end{align}
Multiplying both sides  with $y_i^k-{y_i^\star}^k$, we obtain,
\begin{align}\label{lemma1Result0}
\langle \lambda_i^k + s^k-{\lambda_i^\star}^k, y_i^k-{y_i^\star}^k\rangle = \langle (H_i^k+\alpha I){y_i^\star}^k-y_i^k, y_i^k-{y_i^\star}^k\rangle
\end{align}
Since $H_i^k$ is a positive semidefinite. i.e.,  $\langle H_i^k({y_i^\star}^k-y_i^k), y_i^k-{y_i^\star}^k\rangle \leq 0$, we can re-write
\eqref{lemma1Result0} as
\begin{align}\label{lemma1Result1}
\langle \lambda_i^k + s^k-{\lambda_i^\star}^k, y_i^k-{y^\star}^k\rangle \leq -\alpha \|y_i^k-{y_i^\star}^k\|^2
\end{align}
Using ${y_i^\star}^k={y^\star}^k$, and summing over all clients, and we obtain
\begin{align}\label{lemma1ResultFinal}
\sum_{i=1}^n\langle \lambda_i^k + s^k-{\lambda_i^\star}^k, y_i^k-{y^\star}^k\rangle \leq -\alpha \sum_{i=1}^n\|y_i^k-{y^\star}^k\|^2
\end{align}
That concludes the proof.
\section{Proof of Lemma \ref{lemma_2}}\label{proof_lemma_2}
We start with the statement of Lemma \ref{lemma_1} and multiply both sides of \eqref{lemma1ResultFinal} by $2$ to obtain
\begin{align}\label{main0}
2 A + 2 B \leq  -2\alpha \sum_{i=1}^n\|y_i^k-{y^\star}^k\|^2,
\end{align}
where $A := \sum_{i=1}^n \langle  \lambda_i^k -{\lambda_i^\star}^k, y_i^k-{y^\star}^k\rangle$, and $B := \sum_{i=1}^n \langle  s^k, y_i^k-{y^\star}^k \rangle$. First, we focus on the first term on the left side of \eqref{main0}.
Note that since $\sum_{i=1}^n\lambda_i^k=\sum_{i=1}^n{\lambda_i^\star}^k=\bm{0}$, term $A$ can be written as $A=\sum_{i=1}^n \langle  \lambda_i^k -{\lambda_i^\star}^k, y_i^k\rangle$. Hence, we can write
\begin{align}\label{re}
\nonumber 2 A &= 2 \sum_{i=1}^n \langle  \lambda_i^k -{\lambda_i^\star}^k, y_i^{k}\rangle   \\
\nonumber &\stackrel{\mathrm{(a)}}{=} 2 \sum_{i=1}^n \langle  \lambda_i^{k-1} + \rho y_i^{k}-\rho y^{k} -{\lambda_i^\star}^k, y_i^{k}\rangle \\
\nonumber &= 2 \sum_{i=1}^n \langle  \lambda_i^{k-1}-\rho y^{k} -{\lambda_i^\star}^k, y_i^{k}\rangle + 2 \rho \sum_{i=1}^n \|y_i^{k}\|^2 \\
\nonumber &\stackrel{\mathrm{(b)}}{=} \frac{2}{\rho} \sum_{i=1}^n \langle  \lambda_i^{k-1} -\rho y^{k} -{\lambda_i^\star}^k, \lambda_i^k - \lambda_i^{k-1}+ \rho y^k\rangle+ \rho \sum_{i=1}^n  \|y_i^{k}\|^2 + \rho \sum_{i=1}^n \|y_i^{k}\|^2\\
\nonumber &= \frac{2}{\rho} \sum_{i=1}^n \langle  \lambda_i^{k-1} -\rho y^{k} -{\lambda_i^\star}^k, \lambda_i^k - {\lambda_i^\star}^k + {\lambda_i^\star}^k - \lambda_i^{k-1}+ \rho y^k\rangle + \frac{1}{\rho} \sum_{i=1}^n \|\lambda_i^k - \lambda_i^{k-1} + \rho y^k\|^2 +\rho \sum_{i=1}^n  \|y_i^{k}\|^2 \\
\nonumber &= {- \frac{2}{\rho} \sum_{i=1}^n \|\lambda_i^{k-1} - \rho y^k - {\lambda_i^\star}^k \|^2} + \frac{2}{\rho} \sum_{i=1}^n \langle  \lambda_i^{k-1} -\rho y^{k} -{\lambda_i^\star}^k, \lambda_i^k - {\lambda_i^\star}^k \rangle\\
& + \frac{1}{\rho} \sum_{i=1}^n \|\lambda_i^k - \lambda_i^{k-1} + \rho y^k\|^2 +\rho \sum_{i=1}^n \|y_i^{k}\|^2,
\end{align}
where we used the update of the dual variables, i.e. $\lambda_i^k = \lambda_i^{k-1} + \rho y_i^{k} - \rho y^{k} $ in $\mathrm{(a)}$, and replaced $y_i^{k}$ by $(\lambda_i^k - \lambda_i^{k-1} + \rho y^k)/\rho$ in the first two terms of $\mathrm{(b)}$. Now, we use $\lambda_i^k - \lambda_i^{k-1} = (\lambda_i^k - {\lambda_i^\star}^k)-(\lambda_i^{k-1} - {\lambda_i^\star}^k)$ in the third term of \eqref{re} to write
\begin{align}\label{ee}
\nonumber &\frac{1}{\rho} \sum_{i=1}^n \|\lambda_i^k - \lambda_i^{k-1} + \rho y^k\|^2 \\
\nonumber &=  \frac{1}{\rho} \sum_{i=1}^n \|\lambda_i^k - {\lambda_i^\star}^k - \left(\lambda_i^{k-1} -  {\lambda_i^\star}^k - \rho y^k \right)\|^2\\
&= \frac{1}{\rho} \sum_{i=1}^n \|\lambda_i^k - {\lambda_i^\star}^k \|^2 + \frac{1}{\rho} \sum_{i=1}^n \|\lambda_i^{k-1} -  {\lambda_i^\star}^k - \rho y^k\|^2 - \frac{2}{\rho} \sum_{i=1}^n \langle \lambda_i^{k-1} -  {\lambda_i^\star}^k - \rho y^k  , \lambda_i^k - {\lambda_i^\star}^k\rangle.
\end{align}
Utilizing the expression in \eqref{ee} into \eqref{re}, we get
\begin{align}\label{main1_0}
2 A &= \frac{1}{\rho} \sum_{i=1}^n \|\lambda_i^k - {\lambda_i^\star}^k\|^2 - \frac{1}{\rho} \sum_{i=1}^n \|\lambda_i^{k-1} - {\lambda_i^\star}^k - \rho y^k\|^2 + \rho \sum_{i=1}^n  \|y_i^{k}\|^2\nonumber
\\
 &= \frac{1}{\rho} \sum_{i=1}^n \|\lambda_i^k - {\lambda_i^\star}^k\|^2 - \frac{1}{\rho} \sum_{i=1}^n \|\lambda_i^{k-1} - {\lambda_i^\star}^k\|^2 - \rho n \|y^k\|^2 + \rho \sum_{i=1}^n  \|y_i^{k}\|^2
\end{align}

Next, we tackle the term $B$. Replacing the dual residual $s^{k+1}$ by its definition, we get
\begin{align}
 \nonumber 2 B &= 2 \rho \sum_{i=1}^n \langle y^{k} - y^{k-1}, y_i^k-{y^\star}^k \rangle = 2 \rho \sum_{i=1}^n \langle y^{k} - y^{k-1}, y_i^{k}-y^k + y^{k} - {y^\star}^k\rangle \\
& = 2 \rho \sum_{i=1}^n \langle y^{k} - y^{k-1}, r_i^{k}\rangle + 2 \rho n \langle y^{k}  - y^{k-1}, y^{k}-{y^\star}^k\rangle,
\end{align}
where we utilized the definition $r_i^k=y_i^k-y^k$. 
Using $y^{k}-{y^\star}^k = y^{k} - y^{k-1} + y^{k-1}-{y^\star}^k$, we can write
\begin{align}
2 B = 2 \rho \sum_{i=1}^n \langle y^{k} - y^{k-1}, r_i^{k}\rangle + 2 \rho n \|y^{k} - y^{k-1}\|^2 + 2 \rho n \langle y^{k} - y^{k-1}, y^{k-1}-{y^\star}^k\rangle.
\end{align}
Next, using $y^{k}-y^{k-1} = y^{k} - {y^\star}^k -( y^{k-1}-{y^\star}^k)$, we can write
\begin{align}\label{main02}
\nonumber 2 B&= 2 \rho \sum_{i=1}^n \langle y^{k} - y^{k-1}, r_i^{k}\rangle + 2 \rho n \|y^{k} - y^{k-1}\|^2
 - 2 \rho \| y^{k-1} - {y^\star}^k\|^2 + 2 \rho n \langle y^k-{y^\star}^k, y^{k-1}-{y^\star}^k\rangle \\
\nonumber &= 2 \rho \sum_{i=1}^n \langle y^{k} - y^{k-1}, r_i^{k}\rangle + \rho n \|(y^{k} - {y^\star}^k) - (y^{k-1}-{y^\star}^k)\|^2 + \rho n \|y^{k} - y^{k-1}\|^2
- 2 \rho \| y^{k-1} - {y^\star}^k\|^2\\
&\quad+ 2 \rho n \langle y^k-{y^\star}^k, y^{k-1}-{y^\star}^k\rangle \\
\nonumber &= \rho n \|y^{k} - y^{k-1}\|^2 + \rho n \|y^{k}-{y^\star}^k \|^2-\rho n \|y^{k-1}-{y^\star}^k\|^2 + 2 \rho \sum_{i=1}^n \langle y^{k} - y^{k-1}, r_i^{k}\rangle.
\end{align}
Using the definition of $r_i^{k}$ and the equality in \eqref{updatePS3}, we have
\begin{align}\label{eqq}
\sum_{i=1}^n \langle y^{k} - y^{k-1}, r_i^{k}\rangle
 &= \langle y^{k} - y^{k-1}, \sum_{i=1}^n r_i^{k}\rangle = \langle y^{k} - y^{k-1}, \sum_{i=1}^n y_i^{k} - n y^{k}\rangle = 0.
\end{align}
Hence, from \eqref{main02}, we obtain
\begin{align}\label{main2}
2 B &= \rho n \|y^{k} - y^{k-1}\|^2 + \rho n \|y^{k}-{y^\star}^k \|^2-\rho n \|y^{k-1}-{y^\star}^k\|^2.
\end{align}
Substituting \eqref{main1_0} and \eqref{main02} into \eqref{main0} and rearrange terms, we obtain, 
\begin{align}\label{combinedAB}
&\frac{1}{\rho} \sum_{i=1}^n \|\lambda_i^k- {\lambda_i^\star}^k\|^2  + \rho n \|y^{k}-{y^\star}^k \|^2
\\
&
 \leq \frac{1}{\rho} \sum_{i=1}^n \|\lambda_i^{k-1} - {\lambda_i^\star}^k\|^2+\rho n \|y^{k-1}-{y^\star}^k\|^2-\rho n \|y^{k} - y^{k-1}\|^2+ \rho n \|y^k\|^2 - \rho \sum_{i=1}^n  \|y_i^{k}\|^2-2\alpha \sum_{i=1}^n\|y_i^k-{y^\star}^k\|^2\nonumber
\end{align}
Using $n\sum_{i=1}^n  \|y_i^{k}\|^2 \geq   \|\sum_{i=1}^n y_i^{k}\|^2$, we can easily show that $\rho \sum_{i=1}^n  \|y_i^{k}\|^2 \geq \rho n \|y^k\|^2$, so both terms cancel from the RHS of \eqref{combinedAB}, and we obtain
\begin{align}\label{}
&\frac{1}{\rho} \sum_{i=1}^n \|\lambda_i^k- {\lambda_i^\star}^k\|^2  + \rho n \|y^{k}-{y^\star}^k \|^2
\nonumber\\
&
 \leq \frac{1}{\rho} \sum_{i=1}^n \|\lambda_i^{k-1}- {\lambda_i^\star}^k\|^2+\rho n \|y^{k-1}-{y^\star}^k\|^2-\rho n \|y^{k} - y^{k-1}\|^2-2\alpha \sum_{i=1}^n \|y_i^k-{y^\star}^k\|^2.
\end{align}
Adding and subtracting $\lambda_i^{k-1}$, we get
\begin{align}\label{}
&\frac{1}{\rho} \sum_{i=1}^n \|\lambda_i^k- {\lambda_i^\star}^k\|^2  + \rho n \|y^{k}-{y^\star}^k \|^2
\nonumber\\
&
 \leq \frac{1}{\rho} \sum_{i=1}^n \|\lambda_i^{k-1} -{\lambda_i^\star}^{k-1}+{\lambda_i^\star}^{k-1}- {\lambda_i^\star}^k\|^2+\rho n \|y^{k-1}-{y^\star}^k\|^2-\rho n \|y^{k} - y^{k-1}\|^2-2\alpha \sum_{=1}^n \|y_i^k-{y^\star}^k\|^2
\end{align}
Using $\|a+b\|^2 \leq 2\|a\|^2+2\|b\|^2$, the following holds
\begin{align}\label{}
&\frac{1}{\rho} \sum_{i=1}^n \|\lambda_i^k- {\lambda_i^\star}^k\|^2  + \rho n \|y^{k}-{y^\star}^k \|^2
\\
&
 \leq \frac{2}{\rho} \sum_{i=1}^n \|\lambda_i^{k-1} -{\lambda_i^\star}^{k-1}\|^2+\frac{2}{\rho} \sum_{i=1}^n\|{\lambda_i^\star}^{k-1}- {\lambda_i^\star}^k\|^2+\rho n \|y^{k-1}-{y^\star}^k\|^2-\rho n \|y^{k} - y^{k-1}\|^2-2\alpha \sum_{=1}^n \|y_i^k-{y^\star}^k\|^2\nonumber.
\end{align}
Using ${\lambda_i^\star}^k = g_i^{k} - (H_i^{k}+\alpha^{k} I) {y_i^\star}^{k}$, we get
\begin{align}\label{eq56}
&\frac{1}{\rho} \sum_{i=1}^n \|\lambda_i^k- {\lambda_i^\star}^k\|^2  + \rho n \|y^{k}-{y^\star}^k \|^2
\nonumber\\
&
 \leq \frac{2}{\rho} \sum_{i=1}^n \|\lambda_i^{k-1} -{\lambda_i^\star}^{k-1}\|^2+\frac{2}{\rho} \sum_{i=1}^n\|g_i^{k-1} - (H_i^{k-1}+\alpha^{k-1} I) {y_i^\star}^{k-1}-g_i^{k} + (H_i^{k}+\alpha^{k} I) {y_i^\star}^{k}\|^2\nonumber\\
 &\quad+\rho n \|y^{k-1}-{y^\star}^k\|^2-\rho n \|y^{k} - y^{k-1}\|^2-2\alpha \sum_{=1}^n \|y_i^k-{y^\star}^k\|^2.
\end{align}
Using the definition of $Q_i(\cdot,\cdot)$, we write \eqref{eq56} as
\begin{align}\label{eq57}
&\frac{1}{\rho} \sum_{i=1}^n \|\lambda_i^k- {\lambda_i^\star}^k\|^2  + \rho n \|y^{k}-{y^\star}^k \|^2
\nonumber\\
&
 \leq \frac{2}{\rho} \sum_{i=1}^n \|\lambda_i^{k-1} -{\lambda_i^\star}^{k-1}\|^2+\frac{2}{\rho} \sum_{i=1}^n\|\nabla Q_i(x^{k-1}, {y_i^\star}^{k-1})-\nabla Q_i(x^k, {y_i^\star}^{k})\|^2\nonumber\\
 &\quad+\rho n \|y^{k-1}-{y^\star}^k\|^2-\rho n \|y^{k} - y^{k-1}\|^2-2\alpha \sum_{=1}^n \|y_i^k-{y^\star}^k\|^2.
\end{align}
Using the lipschitz continuity of $\nabla Q$, we obtain
\begin{align}\label{eq58}
&\frac{1}{\rho} \sum_{i=1}^n \|\lambda_i^k- {\lambda_i^\star}^k\|^2  + \rho n \|y^{k}-{y^\star}^k \|^2
\nonumber\\
\nonumber &
 \leq \frac{2}{\rho} \sum_{i=1}^n \|\lambda_i^{k-1} -{\lambda_i^\star}^{k-1}\|^2+\frac{2L_q^2}{\rho} \sum_{i=1}^n\| {y_i^\star}^{k-1}- {y_i^\star}^{k}\|^2+\rho n \|y^{k-1}-{y^\star}^k\|^2\\
 &-\rho n \|y^{k} - y^{k-1}\|^2-2\alpha \sum_{=1}^n \|y_i^k-{y^\star}^k\|^2.
\end{align}
%
%Using $\sum_{i=1}^n\| {y_i^\star}^{k-1}- {y_i^\star}^{k}\|^2 \leq \beta \| {y^\star}^{k-1}- {y^\star}^{k}\|^2$, we %get
%\begin{align}\label{}
%&\frac{1}{\rho} \sum_{i=1}^n \|\lambda_i^k- {\lambda_i^\star}^k\|^2  + \rho n \|y^{k}-{y^\star}^k \|^2
%\nonumber\\
%&
% \leq \frac{2}{\rho} \sum_{i=1}^n \|\lambda_i^{k-1} -{\lambda_i^\star}^{k-1}\|^2+\frac{2\beta L_q^2n}{\rho}\| {y^\star}^{k-1}- {y^\star}^{k}\|^2+\rho n \|y^{k-1}-{y^\star}^k\|^2-\rho n \|y^{k} - y^{k-1}\|^2-2\alpha n \|{y^\star}^k-y^{k}\|^2
%\end{align}
%
Equivalently, we can write \eqref{eq58} as
\begin{align}\label{}
&\frac{1}{\rho} \sum_{i=1}^n \|\lambda_i^k- {\lambda_i^\star}^k\|^2  + \rho n \|y^{k}-{y^\star}^k \|^2
\nonumber\\
&
 \leq \frac{1}{\rho} \sum_{i=1}^n \|\lambda_i^{k-1} -{\lambda_i^\star}^{k-1}\|^2+\frac{1}{\rho} \sum_{i=1}^n \|g_i^{k-1} -s^{k-1}- (H_i^{k-1}+\alpha^{k-1} I) y_i^{k-1}-g_i^{k-1} + (H_i^{k-1}+\alpha^{k-1} I) {y_i^\star}^{k-1}\|^2\nonumber\\
 &\quad+\frac{2L_q^2}{\rho} \sum_{i=1}^n\| {y_i^\star}^{k-1}- {y_i^\star}^{k}\|^2+\rho n \|y^{k-1}-{y^\star}^k\|^2-\rho n \|y^{k} - y^{k-1}\|^2-2\alpha \sum_{=1}^n \|y_i^k-{y^\star}^k\|^2.
\end{align}
Using the inequality $\|a+b\|^2 \leq 2\|a\|^2+2\|b\|^2$ and the expression of $\nabla Q$, we obtain
\begin{align}\label{}
&\frac{1}{\rho} \sum_{i=1}^n \|\lambda_i^k- {\lambda_i^\star}^k\|^2  + \rho n \|y^{k}-{y^\star}^k \|^2
\nonumber\\
&
 \leq \frac{1}{\rho} \sum_{i=1}^n \|\lambda_i^{k-1} -{\lambda_i^\star}^{k-1}\|^2+\frac{2}{\rho} \sum_{i=1}^n \|\nabla Q_i(x^{k-1},y_i^{k-1})-\nabla Q_i(x^{k-1},{y_i^\star}^{k-1})\|^2+\frac{2n}{\rho}\|s^{k-1}\|^2\nonumber\\
 \nonumber &\quad+\frac{2L_q^2}{\rho} \sum_{i=1}^n\| {y_i^\star}^{k-1}- {y_i^\star}^{k}\|^2+\rho n \|y^{k-1}-{y^\star}^k\|^2-\rho n \|y^{k} - y^{k-1}\|^2-2\alpha \sum_{=1}^n \|y_i^k-{y^\star}^k\|^2\\
&
 \leq \frac{1}{\rho} \sum_{i=1}^n \|\lambda_i^{k-1} -{\lambda_i^\star}^{k-1}\|^2+\frac{2 L_q^2}{\rho}  \sum_{i=1}^n\|y_i^{k-1}-{y^\star}^{k-1}\|^2+\frac{2n}{\rho}\|s^{k-1}\|^2+\frac{2 L_q^2}{\rho}\sum_{i=1}^n\| {y^\star}^{k-1}- {y^\star}^{k}\|^2\nonumber\\
 &\quad+\rho n \|y^{k-1}-{y^\star}^k\|^2-\rho n \|y^{k} - y^{k-1}\|^2-2\alpha \sum_{=1}^n \|y_i^k-{y^\star}^k\|^2.
\end{align}
%
%\begin{align}\label{}
%&\frac{1}{\rho} \sum_{i=1}^n \|\lambda_i^k- {\lambda_i^\star}^k\|^2  + \rho n \|y^{k}-{y^\star}^k \|^2
%\nonumber\\
%&
 %\leq \frac{1}{\rho} \sum_{i=1}^n \|\lambda_i^{k-1} -{\lambda_i^\star}^{k-1}\|^2+\frac{2\beta L_q^2 n}{\rho}  \|y^{k-1}-{y^\star}^{k-1}\|^2+\frac{2n}{\rho}\|s^{k-1}\|^2+\frac{2\beta L_q^2n}{\rho}\| {y^\star}^{k-1}- {y^\star}^{k}\|^2\nonumber\\
 %&+\rho n \|y^{k-1}-{y^\star}^{k}\|^2-\rho n \|y^{k} - y^{k-1}\|^2-2\alpha n %\|y^{k}-{y^\star}^k\|^2
%\end{align}
%
Replacing $s^{k-1}$ by its definition, we get
\begin{align}\label{}
&\frac{1}{\rho} \sum_{i=1}^n \|\lambda_i^k- {\lambda_i^\star}^k\|^2  + \rho n \|y^{k}-{y^\star}^k \|^2
\nonumber\\
&
 \leq \frac{1}{\rho} \sum_{i=1}^n \|\lambda_i^{k-1} -{\lambda_i^\star}^{k-1}\|^2+\frac{2 L_q^2}{\rho}  \sum_{i=1}^n\|y_i^{k-1}-{y^\star}^{k-1}\|^2+2n\rho\|y^{k-1}-y^{k-2}\|^2+\frac{2 L_q^2n}{\rho}\| {y^\star}^{k-1}- {y^\star}^{k}\|^2\nonumber\\
 &\quad+\rho n \|y^{k-1}-{y^\star}^{k}\|^2-\rho n \|y^{k} - y^{k-1}\|^2-2\alpha \sum_{i=1}^n \|y_i^{k}-{y^\star}^k\|^2.
\end{align}
%
%
%\begin{align}\label{}
%&\frac{1}{\rho} \sum_{i=1}^n \|\lambda_i^k- {\lambda_i^\star}^k\|^2  + \rho n \|y^{k}-{y^\star}^k \|^2
%\nonumber\\
%&
% \leq \frac{1}{\rho} \sum_{i=1}^n \|\lambda_i^{k-1} -{\lambda_i^\star}^{k-1}\|^2+\frac{2\beta L_q^2 n}{\rho} \|y^{k-1}-{y^\star}^{k-1}\|^2+2\rho n\|y^{k-1}-y^{k-2}\|^2+\frac{2\beta L_q^2n}{\rho}\| {y^\star}^{k-1}- {y^\star}^{k}\|^2\nonumber\\
%  &+2\rho n \|y^{k-1}-{y^\star}^{k-1}\|^2+2\rho n\|{y^\star}^{k-1}-{y^\star}^k\|^2-\rho n \|y^{k} - y^{k-1}\|^2-\alpha n \|y^{k}-{y^\star}^k\|^2
%\end{align}
%
Let $\alpha = \alpha_1 + \alpha_2$. Adding and subtracting $y^k$ in $\|y^{k-1}-{y^\star}^k\|^2$ and using $\|a+b\|^2 \leq 2\|a\|^2+2\|b\|^2$, we obtain
\begin{align}\label{eq62}
&\frac{1}{\rho} \sum_{i=1}^n \|\lambda_i^k- {\lambda_i^\star}^k\|^2  + \rho n \|y^{k}-{y^\star}^k \|^2
\nonumber\\
&
 \leq \frac{1}{\rho} \sum_{i=1}^n \|\lambda_i^{k-1} -{\lambda_i^\star}^{k-1}\|^2+\frac{2 L_q^2}{\rho} \sum_{i=1}^n\|y_i^{k-1}-{y^\star}^{k-1}\|^2+2\rho n\|y^{k-1}-y^{k-2}\|^2+\frac{2 L_q^2n}{\rho}\| {y^\star}^{k-1}- {y^\star}^{k}\|^2\nonumber\\
 &\quad+2\rho n \|y^k-y^{k-1}\|^2+2\rho n\|y^k-{y^\star}^k\|^2-\rho n \|y^{k} - y^{k-1}\|^2-2\alpha_1 \sum_{i=1}^n \|y_i^{k}-{y^\star}^k\|^2-2\alpha_2 \sum_{i=1}^n \|y_i^{k}-{y^\star}^k\|^2.
\end{align}
 Using $\sum_{i=1}^n \|y_i^{k}-{y^\star}^k\|^2 \geq  \|\sum_{i=1}^n(y_i^{k}-{y^\star}^k)\|^2=  n \|y^{k}-{y^\star}^k\|^2 $, we can rewrite \eqref{eq62} as
 \begin{align}\label{}
&\frac{1}{\rho} \sum_{i=1}^n \|\lambda_i^k- {\lambda_i^\star}^k\|^2  + \rho n \|y^{k}-{y^\star}^k \|^2
\nonumber\\
&
 \leq \frac{1}{\rho} \sum_{i=1}^n \|\lambda_i^{k-1} -{\lambda_i^\star}^{k-1}\|^2+\frac{2 L_q^2}{\rho}\sum_{i=1}^n \|y_i^{k-1}-{y^\star}^{k-1}\|^2+2\rho n\|y^{k-1}-y^{k-2}\|^2+\frac{2 L_q^2n}{\rho}\| {y^\star}^{k-1}- {y^\star}^{k}\|^2\nonumber\\
 &\quad+2\rho n \|y^k-y^{k-1}\|^2+2\rho n\|y^k-{y^\star}^k\|^2-\rho n \|y^{k} - y^{k-1}\|^2-2\alpha_1 n \|y^{k}-{y^\star}^k\|^2-2\alpha_2 \sum_{i=1}^n \|y_i^{k}-{y^\star}^k\|^2.
\end{align}
 Assuming $\|y^{k-1}-y^k\|^2 \leq \|y^{k}-{y^\star}^k\|^2$ which holds for sufficiently large $\rho$, and choosing $\alpha_1 \geq 2.5\rho$, we get
\begin{align}\label{}
&\frac{1}{\rho} \sum_{i=1}^n \|\lambda_i^k- {\lambda_i^\star}^k\|^2  + \rho n \|y^{k}-{y^\star}^k \|^2
\nonumber\\
&
 \leq \frac{1}{\rho} \sum_{i=1}^n \|\lambda_i^{k-1} -{\lambda_i^\star}^{k-1}\|^2+\frac{2 L_q^2}{\rho}\sum_{i=1}^n \|y_i^{k-1}-{y^\star}^{k-1}\|^2+2\rho n\|y^{k-1}-y^{k-2}\|^2+\frac{2 L_q^2n}{\rho}\| {y^\star}^{k-1}- {y^\star}^{k}\|^2\nonumber\\
 &\quad-2\rho n \|y^{k} - y^{k-1}\|^2-2\alpha_2 \sum_{i=1}^n \|y^{k}-{y^\star}^k\|^2.
\end{align}
Re-arranging the terms, we get
\begin{align}\label{}
&\frac{1}{\rho} \sum_{i=1}^n \|\lambda_i^k- {\lambda_i^\star}^k\|^2  + \rho n \|y^{k}-{y^\star}^k \|^2+2\rho n \|y^{k} - y^{k-1}\|^2
\nonumber\\
&
 \leq \frac{1}{\rho} \sum_{i=1}^n \|\lambda_i^{k-1} -{\lambda_i^\star}^{k-1}\|^2+\frac{2 L_q^2}{\rho}\sum_{i=1}^n \|y_i^{k-1}-{y^\star}^{k-1}\|^2+2\rho n\|y^{k-1}-y^{k-2}\|^2\nonumber\\
 &\quad+\frac{2 L_q^2n}{\rho}\| {y^\star}^{k-1}- {y^\star}^{k}\|^2-2\alpha_2 \sum_{i=1}^n \|y_i^{k}-{y^\star}^k\|^2.
\end{align}
Adding and subtracting $y^{k-1}$ in $\|{y^\star}^{k-1}-{y^\star}^{k}\|^2$, we get
\begin{align}\label{}
&\frac{1}{\rho} \sum_{i=1}^n \|\lambda_i^k- {\lambda_i^\star}^k\|^2  + \rho n \|y^{k}-{y^\star}^k \|^2+2\rho n \|y^{k} - y^{k-1}\|^2
\nonumber\\
&
 \leq \frac{1}{\rho} \sum_{i=1}^n \|\lambda_i^{k-1} -{\lambda_i^\star}^{k-1}\|^2+\frac{2 L_q^2 }{\rho}\sum_{i=1}^n \|y_i^{k-1}-{y^\star}^{k-1}\|^2+2\rho n\|y^{k-1}-y^{k-2}\|^2+\frac{4 L_q^2n}{\rho}\| {y^\star}^{k-1}-y^{k-1}\|^2\nonumber\\
 &\quad+\frac{4 L_q^2n}{\rho}\|y^{k-1}- {y^\star}^{k}\|^2-2\alpha_2 \sum_{i=1}^n \|y_i^{k}-{y^\star}^k\|^2.
\end{align}
Next, let $\alpha_2 = \alpha_3 + \alpha_4$. Adding and subtracting $y^{k}$ in $\|y^{k-1}-{y^\star}^{k}\|^2$, we get
\begin{align}\label{}
&\frac{1}{\rho} \sum_{i=1}^n \|\lambda_i^k- {\lambda_i^\star}^k\|^2  + \rho n \|y^{k}-{y^\star}^k \|^2+2\rho n \|y^{k} - y^{k-1}\|^2
\nonumber\\
&
 \leq \frac{1}{\rho} \sum_{i=1}^n \|\lambda_i^{k-1} -{\lambda_i^\star}^{k-1}\|^2+\frac{2 L_q^2}{\rho}\sum_{i=1}^n \|y_i^{k-1}-{y^\star}^{k-1}\|^2+2\rho n\|y^{k-1}-y^{k-2}\|^2+\frac{4 L_q^2n}{\rho}\| {y^\star}^{k-1}-y^{k-1}\|^2\nonumber\\
 &\quad+\frac{8 L_q^2n}{\rho}\|y^{k-1}-y^k\|^2+\frac{8 L_q^2n}{\rho}\| y^k-{y^\star}^{k}\|^2-2\alpha_3 n \|y^{k}-{y^\star}^k\|^2-2\alpha_4 \sum_{i=1}^n \|y_i^{k}-{y^\star}^k\|^2.
\end{align}
Choosing $\alpha_3 \geq \frac{8 L_q^2n}{\rho}$, and using the assumption $\|y^{k-1}-y^k\|^2 \leq \|y^{k}-{y^\star}^k\|^2$, we get
\begin{align}\label{eq68}
&\frac{1}{\rho} \sum_{i=1}^n \|\lambda_i^k- {\lambda_i^\star}^k\|^2  + \rho n \|y^{k}-{y^\star}^k \|^2+2\rho n \|y^{k} - y^{k-1}\|^2
\nonumber\\
&
 \leq \frac{1}{\rho} \sum_{i=1}^n \|\lambda_i^{k-1} -{\lambda_i^\star}^{k-1}\|^2+\frac{2 L_q^2}{\rho}\sum_{i=1}^n \|y_i^{k-1}-{y^\star}^{k-1}\|^2+2\rho n\|y^{k-1}-y^{k-2}\|^2+\frac{4 L_q^2n}{\rho}\| {y^\star}^{k-1}-y^{k-1}\|^2\nonumber\\
 &\quad-2\alpha_4 \sum_{i=1}^n \|y_i^{k}-{y^\star}^k\|^2.
\end{align}
Let $\alpha_4=\alpha_5+\alpha_6$, we write \eqref{eq68} as
\begin{align}\label{}
&\frac{1}{\rho} \sum_{i=1}^n \|\lambda_i^k- {\lambda_i^\star}^k\|^2  + \rho n \|y^{k}-{y^\star}^k \|^2+2\rho n \|y^{k} - y^{k-1}\|^2
\nonumber\\
&
 \leq \frac{1}{\rho} \sum_{i=1}^n \|\lambda_i^{k-1} -{\lambda_i^\star}^{k-1}\|^2+\frac{2 L_q^2}{\rho}\sum_{i=1}^n \|y_i^{k-1}-{y^\star}^{k-1}\|^2+2\rho n\|y^{k-1}-y^{k-2}\|^2+\frac{4 L_q^2n}{\rho}\|y^{k-1}-{y^\star}^{k-1}\|^2\nonumber\\
 &\quad-2\alpha_5 \sum_{i=1}^n \|y_i^{k}-{y^\star}^k\|^2-2\alpha_6 \sum_{i=1}^n \|y_i^{k}-{y^\star}^k\|^2.
\end{align}
Re-arrange terms, we obtain
\begin{align}\label{eq70}
&\frac{1}{\rho} \sum_{i=1}^n \|\lambda_i^k- {\lambda_i^\star}^k\|^2+2\alpha_5 \sum_{i=1}^n \|y_i^{k}-{y^\star}^k\|^2  + \rho n \|y^{k}-{y^\star}^k \|^2+2\rho n \|y^{k} - y^{k-1}\|^2
\nonumber\\
&
 \leq \frac{1}{\rho} \sum_{i=1}^n \|\lambda_i^{k-1} -{\lambda_i^\star}^{k-1}\|^2+\frac{2 L_q^2}{\rho}\sum_{i=1}^n \|y_i^{k-1}-{y^\star}^{k-1}\|^2+\frac{4 L_q^2n}{\rho}\|y^{k-1}-{y^\star}^{k-1}\|^2+2\rho n\|y^{k-1}-y^{k-2}\|^2\nonumber\\
 &\quad-2\alpha_6 \sum_{i=1}^n \|y_i^{k}-{y^\star}^k\|^2.
\end{align}
Let $\beta_1=\alpha_5$, and $\beta_2=\alpha_6$, Hence, we can write \eqref{eq70} as
\begin{align}\label{lemma2Result}
&\frac{1}{\rho} \sum_{i=1}^n \|\lambda_i^k- {\lambda_i^\star}^k\|^2+2\beta_1 \sum_{i=1}^n \|y_i^{k}-{y^\star}^k\|^2  + \rho n \|y^{k}-{y^\star}^k \|^2+2\rho n \|y^{k} - y^{k-1}\|^2
\nonumber\\
&
 \leq \frac{1}{\rho} \sum_{i=1}^n \|\lambda_i^{k-1} -{\lambda_i^\star}^{k-1}\|^2+\frac{2 L_q^2}{\rho}\sum_{i=1}^n \|y_i^{k-1}-{y^\star}^{k-1}\|^2+\frac{4 L_q^2n}{\rho}\|y^{k-1}-{y^\star}^{k-1}\|^2+2\rho n\|y^{k-1}-y^{k-2}\|^2\nonumber\\
 &\quad-2\beta_2 \sum_{i=1}^n \|y_i^{k}-{y^\star}^k\|^2.
\end{align}
%e
Note that,
\begin{align}
\alpha=&\alpha_1+\alpha_2\nonumber\\
=&\alpha_1+\alpha_3+\beta_1+\beta_2\nonumber\\
\geq& 2.5 \rho + \frac{8L_q^2n}{\rho}+\beta_1+\beta_2
\end{align}
Hence,
%
%\begin{align}
$\beta_1+\beta_2\leq \alpha - 2.5 \rho - \frac{8L_q^2n}{\rho}$. 
%\end{align}
%
That concludes the proof.

\section{Proof of Theorem \ref{theorem_1}}\label{proof_of_theorem}
From the statement of Lemma \ref{lemma_2}, we can write 
\begin{align}\label{lemma2Result2}
\frac{1}{\rho}& \sum_{i=1}^n \|\lambda_i^k- {\lambda_i^\star}^k\|^2+2\beta_1 \sum_{i=1}^n \|y_i^{k}-{y^\star}^k\|^2  + \rho n \|y^{k}-{y^\star}^k \|^2+2\rho n \|y^{k} - y^{k-1}\|^2
\nonumber\\
&
 \leq \frac{1}{\rho} \sum_{i=1}^n \|\lambda_i^{k-1} -{\lambda_i^\star}^{k-1}\|^2+\frac{2 L_q^2}{\rho}\sum_{i=1}^n \|y_i^{k-1}-{y^\star}^{k-1}\|^2
+\frac{4 L_q^2n}{\rho}\|y^{k-1}-{y^\star}^{k-1}\|^2+2\rho n\|y^{k-1}-y^{k-2}\|^2
\nonumber
\\
&\quad -2\beta_2 \sum_{i=1}^n \|y_i^{k}-{y^\star}^k\|^2.
\end{align}
Choosing $\alpha$ that satisfies \eqref{alphaCondition} for $\beta_1\geq \frac{L_q^2}{\rho}$, $\rho\geq 2L_q$, and $\beta_2 > 0$ and from the definition of Lyapunov function $V_k$ \eqref{Lyapunov}, we can write
\begin{align}\label{them1inq11}
V^k
&\leq V^{k-1}-\left(2\beta_2 \sum_{i=1}^n \|y_i^{k}-{y^\star}^k\|^2\right).
\end{align}
Therefore, $V^k$ decreases in each iteration $k$. 
%Next, we note that $\|y_i^{k}-{y^\star}^k\|$ is the optimal direction (cf. \eqref{updateLocal2}) and is zero only when $x^k=x^*$ and error $\|y_i^{k}-{y^\star}^k\|$ is zero. Otherwise there always exists a $\epsilon>0$ such that $\|y_i^{k}-{y^\star}^k\|\geq \epsilon$. This shows that $V^k$ is a monotonically decreasing sequence and since we know that $V^k$ is a positive sequence, then using the monotone convergence theorem, we get that $V^k \rightarrow 0$ as $k \rightarrow \infty$. 
Consequently, since $V_k\geq 0$, this implies that every term in $V^k$ goes to $0$, i.e. $\lambda_i^k \rightarrow {\lambda_i^\star}^k$, $y_i^{k} \rightarrow {y^\star}^k$, and $y^{k} \rightarrow {y^\star}^k$, 
%Since our directions to update $x^{k+1}$ converge to optimal directions, this would eventually imply that $x^{k} \rightarrow x^\star$ as $k \rightarrow \infty$, 
which completes the proof.

\if0
\begin{align}\label{lemma2FinalInq}
  \frac{1}{\rho} \sum_{i=1}^n \|\lambda_i^k - \lambda_i^\star\|^2  +\rho n\|y^k\|^2
\leq &  \frac{1}{\rho} \sum_{i=1}^n \|\lambda_i^{k-1} - \lambda_i^\star\|^2+\rho n \|x^{k}-x^{k-1}\|^2-3\rho n \|y^{k}\|^2-\rho n \|x^{k+1}-x^{k-1}\|^2
\nonumber\\&- \rho \sum_{i=1}^n  \|y_i^{k}\|^2+\eta L^2 n \|x^k-x^\star\|^2+\frac{1}{\eta} \sum_{i=1}^n \|y_i^k\|^2.
\end{align}

Using $y^k=x^{k+1}-x^{k}$ and $y^{k-1}=x^{k}-x^{k-1}$, we get

\begin{align}\label{lemma2FinalInq}
  \frac{1}{\rho} \sum_{i=1}^n \|\lambda_i^k - \lambda_i^\star\|^2  +\rho n\|y^{k}\|^2
\leq&  \frac{1}{\rho} \sum_{i=1}^n \|\lambda_i^{k-1} - \lambda_i^\star\|^2+\rho n \|y^{k-1}\|^2-3\rho n \|y^{k}\|^2-\rho n \|x^{k+1}-x^{k-1}\|^2
\nonumber\\&- \rho \sum_{i=1}^n  \|y_i^{k}\|^2+\eta L^2 n \|x^k-x^\star\|^2+\frac{1}{\eta} \sum_{i=1}^n \|y_i^k\|^2.
\end{align}

%\begin{align}\label{lemma2FinalInq}
%  \frac{1}{\rho} \sum_{i=1}^N \|\lambda_i^k - \lambda_i^\star\|^2  +\rho N\|x^{k+1}-x^{k}\|^2
%\leq&  \frac{1}{\rho} \sum_{i=1}^N \|\lambda_i^{k-1} - \lambda_i^\star\|^2+\rho N\|x^{k}-x^{k-1}\|^2\nonumber\\
%&-3\rho N \|y^{k}\|^2-\rho N\|x^{k+1} - x^{k-1}\|^2
%\nonumber\\&- \rho \sum_{i=1}^N  \|y_i^{k}\|^2+\eta L^2N \|x^k-x^\star\|^2+\frac{1}{\eta} \sum_{i=1}^N \|y_i^k\|^2
%\end{align}

\fi

\if0

Adding \eqref{lemma2FinalInq} and \eqref{lemm3_fin}, we get
\begin{align}\label{them1inq1}
\nonumber \frac{1}{\rho} \sum_{i=1}^n \|\lambda_i^k - \lambda_i^\star\|^2  &+\rho n \|y^{k}\|^2+\|x^{k+1} - x^\star\|^2\\
\leq& \frac{1}{\rho} \sum_{i=1}^n \|\lambda_i^{k-1} - \lambda_i^\star\|^2+\rho n \|y^{k-1}\|^2-3\rho n \|y^{k}\|^2-\rho n \|x^{k+1} - x^{k-1}\|^2- \rho \sum_{i=1}^n  \|y_i^{k}\|^2
\nonumber\\ &+\eta L^2 n \|x^k-x^\star\|^2+\frac{1}{\eta} \sum_{i=1}^n \|y_i^k\|^2 +\frac{1}{2} \|x^k-x^\star\|^2+4\| y^k\|^2 - 2\|x^{k+1}-x^{k+1}_{*}\|^2.
\end{align}
Re-arranging the terms, we get
\begin{align}\label{them1inq1}
\nonumber &\frac{1}{\rho} \sum_{i=1}^n \|\lambda_i^k - \lambda_i^\star\|^2  +\rho n \|y^{k}\|^2+\|x^{k+1} - x^\star\|^2\\
\leq &\frac{1}{\rho} \sum_{i=1}^n \|\lambda_i^{k-1} - \lambda_i^\star\|^2+\rho n \|y^{k-1}\|^2+\big(\eta L^2 n +\frac{1}{2}\big) \|x^k-x^\star\|^2-3\rho n \|y^{k}\|^2-\rho n \|x^{k+1} - x^{k-1}\|^2- \rho \sum_{i=1}^n  \|y_i^{k}\|^2
\nonumber\\ &\quad+\frac{1}{\eta} \sum_{i=1}^n \|y_i^k\|^2+4\| y^k\|^2 - 2\|x^{k+1}-x^{k+1}_{*}\|^2.
\end{align}
By setting $\eta=\frac{1}{2L^2n}$, we obtain
\begin{align}\label{them1inq1}
\nonumber \frac{1}{\rho} \sum_{i=1}^n \|\lambda_i^k - \lambda_i^\star\|^2  &\quad+\rho n \|y^{k}\|^2+\|x^{k+1} - x^\star\|^2\\
\leq &\frac{1}{\rho} \sum_{i=1}^n \|\lambda_i^{k-1} - \lambda_i^\star\|^2+\rho n \|y^{k-1}\|^2+\|x^k-x^\star\|^2-3\rho n \|y^{k}\|^2-\rho n \|x^{k+1} - x^{k-1}\|^2- \rho \sum_{i=1}^n  \|y_i^{k}\|^2
\nonumber\\ &\quad+\frac{1}{\eta} \sum_{i=1}^n \|y_i^k\|^2 +4\| y^k\|^2 - 2\|x^{k+1}-x^{k+1}_{*}\|^2.
\end{align}
By choosing $\rho > \max\{\frac{1}{\eta},\frac{4}{3n}\} = 2\max\{ L^2 n,\frac{2}{3n}\}$, we can write
\begin{align}\label{them1inq1}
\nonumber \frac{1}{\rho} \sum_{i=1}^n \|\lambda_i^k - \lambda_i^\star\|^2  &+\rho n \|y^{k}\|^2+\|x^{k+1} - x^\star\|^2\\
&\leq \frac{1}{\rho} \sum_{i=1}^n \|\lambda_i^{k-1} - \lambda_i^\star\|^2+\rho n \|y^{k-1}\|^2+\|x^k-x^\star\|^2-\rho n \|x^{k+1} - x^{k-1}\|^2 - 2\|x^{k+1}-x^{k+1}_{*}\|^2.
\end{align}
\textcolor{red}{we do not need this step now} Since $y^*=0$, we can write
\begin{align}\label{them1inq1}
\nonumber \frac{1}{\rho} \sum_{i=1}^n \|\lambda_i^k - \lambda_i^\star\|^2  &+\rho n \|y^{k}-y^*\|^2+\|x^{k+1} - x^\star\|^2\\
&\leq \frac{1}{\rho} \sum_{i=1}^n \|\lambda_i^{k-1} - \lambda_i^\star\|^2+\rho n \|y^{k-1}-y^*\|^2+\|x^k-x^\star\|^2-\rho n \|x^{k+1} - x^{k-1}\|^2 - 2\|x^{k+1}-x^{k+1}_{*}\|^2.
\end{align}
Defining the Lyapunov function $V^k$ as
\begin{align}
   V^k =  \frac{1}{\rho} \sum_{i=1}^n \|\lambda_i^k - \lambda_i^\star\|^2  +\rho n \|y^{k}-y^*\|^2+\|x^{k+1} - x^\star\|^2,
\end{align}
%\begin{align}\label{them1inq1}
%\nonumber &\frac{1}{\rho} \sum_{i=1}^n \|\lambda_i^k - \lambda_i^\star\|^2  +\rho n \|y^{k}\|^2+\|x^{k+1} - x^\star\|^2\\
%&\leq \frac{1}{\rho} \sum_{i=1}^n \|\lambda_i^{k-1} - \lambda_i^\star\|^2+\rho n \|y^{k-1}\|^2+\|x^k-x^\star\|^2-\rho n \|x^{k+1} - x^{k-1}\|^2 - 2\|x^{k+1}-x^{k+1}_{*}\|^2
%\end{align}
we can write \eqref{them1inq1} as
\begin{align}\label{them1inq11}
V^k
&\leq V^{k-1}-\left(\rho n \|x^{k+1} - x^{k-1}\|^2 + 2\|x^{k+1}-x^{k+1}_{*}\|^2\right).
\end{align}
Therefore, $V^k$ decreases in each iteration $k$. Since we know that $V^k$ is a positive sequence, then using the monotone convergence theorem, we get that $V^k \rightarrow 0$ as $k \rightarrow \infty$. Consequently, every term in $V^k$ goes to $0$, i.e. $\lambda_i^k \rightarrow \lambda_i^\star$, $y^{k} \rightarrow y^\star$, and $x^{k+1} \rightarrow x^\star$ as $k \rightarrow \infty$, which completes the proof.

\textcolor{red}{Hi Anis, I am writing the whole argument here to make it clear how (79) implies the convergence we need. You may take a look and then finalize.}

\textcolor{blue}{Therefore, $V^k$ decreases in each iteration $k$. Now after rearranging the terms in \eqref{them1inq11}, we obtain
\begin{align}\label{them1inq1122}
\left(\rho n \|x^{k+1} - x^{k-1}\|^2 + 2\|x^{k+1}-x^{k+1}_{*}\|^2\right) \leq V^{k-1}-V^k. 
\end{align}
Evaluate the telescopic sum for $k=1$ to $K$, we obtain
\begin{align}\label{them1inq11222}
\sum_{k=1}^K\left(\rho n \|x^{k+1} - x^{k-1}\|^2 + 2\|x^{k+1}-x^{k+1}_{*}\|^2\right) \leq V^{0}, 
\end{align}
where we drop the negative term $-V_{K}$ from the right-hand side. Assuming initialization is such that $V^0$ is finite, then after taking the limit $K\rightarrow\infty$ in \eqref{them1inq11222}, we obtain
\begin{align}\label{them1inq112222}
\lim_{K\rightarrow\infty}\sum_{k=1}^K\left(\rho n \|x^{k+1} - x^{k-1}\|^2 + 2\|x^{k+1}-x^{k+1}_{*}\|^2\right) \leq V^{0}.
\end{align}
Since the left-hand side in \eqref{them1inq112222} in sum of infinite positive terms which is bounded above by a constant, this implies that $\lim_{k\rightarrow\infty} \|x^{k+1} - x^{k-1}\|^2\rightarrow 0$ and  $\lim_{k\rightarrow\infty}\|x^{k+1}-x^{k+1}_{*}\|^2\rightarrow 0$. i.e., it tells that the direction converges to the optimal direction, $\lim_{k\rightarrow\infty}\|y^k-y^*(x^{k})\|^2\rightarrow 0$, and the iterate updates also converge,  $\lim_{k\rightarrow\infty} \|x^{k} - x^{k-1}\|^2\rightarrow 0$. Combining both yilds $\lim_{k\rightarrow\infty} \|x^{k} - x^{*}\|^2\rightarrow 0$, and that concludes the proof.} \textcolor{red}{The last line is not correct according to me. This implies $\|x^{k+1} - x^{k-1}\|^2$ goes to zero, not $\|x^{k} - x^{k-1}\|^2$, are they both equivalent? I don't think so, we need to explicitly prove that.}
\fi

\if0

..\\
..\\
..\\
..\\
..\\
..\\
..\\
..\\
..\\

Adding \eqref{lemma2FinalInq} and \eqref{lemma3FinalInq}, we get
\begin{align}\label{them1inq1}
\nonumber &\frac{1}{\rho} \sum_{i=1}^n \|\lambda_i^k - \lambda_i^\star\|^2  +\rho n \|x^{k+1}-x^{k}\|^2+\|x^{k+1} - x^\star\|^2\\
&\leq \frac{1}{\rho} \sum_{i=1}^n \|\lambda_i^{k-1} - \lambda_i^\star\|^2+\rho n \|x^{k}-x^{k-1}\|^2-3\rho n \|y^{k}\|^2-\rho n \|x^{k+1} - x^{k-1}\|^2- \rho \sum_{i=1}^n  \|y_i^{k}\|^2
\nonumber\\ \nonumber&+\eta L^2 n \|x^k-x^\star\|^2+\frac{1}{\eta} \sum_{i=1}^n \|y_i^k\|^2 +\frac{1}{2}\|x^k-x^\star\|^2 + \frac{2 \delta}{n}\sum_{i=1}^{n}\| {u}_i^k-{u}^\star(x^k)\|^2+  2\frac{L^2}{\mu^2}\| x^k-x^{k-1}\|^2 \\
&\leq  \frac{1}{\rho} \sum_{i=1}^n \|\lambda_i^{k-1} - \lambda_i^\star\|^2+\rho n\|x^{k}-x^{k-1}\|^2 -3\rho n \|y^{k}\|^2-\rho n\|x^{k+1} - x^{k-1}\|^2- \rho_1 \sum_{i=1}^n  \|y_i^{k}\|^2
\nonumber\\&- \rho_2 \sum_{i=1}^n  \|y_i^{k}\|^2+\eta L^2 n \|x^k-x^\star\|^2+\frac{1}{\eta} \sum_{i=1}^n \|y_i^k\|^2+\frac{1}{2}\|x^k-x^\star\|^2 + \frac{2 \delta}{n}\sum_{i=1}^{n}\| {u}_i^k-{u}^\star(x^k)\|^2+  \frac{2L^2}{\mu^2}\| x^k-x^{k-1}\|^2,
\end{align}
where $\rho_1+\rho_2=\rho$. Using the inequality $\|\sum_{i=1}^{n} y_i^k\|^2 \leq n \sum_{i=1}^{n} \| y_i^k\|^2$, we can write
\begin{align}\label{them1inq1}
\nonumber &\frac{1}{\rho} \sum_{i=1}^n \|\lambda_i^k - \lambda_i^\star\|^2  +\rho n\|x^{k+1}-x^{k}\|^2+\|x^{k+1} - x^\star\|^2\\
\nonumber&\leq \frac{1}{\rho} \sum_{i=1}^n \|\lambda_i^{k-1} - \lambda_i^\star\|^2+\rho n\|x^{k}-x^{k-1}\|^2-3\rho n \|y^{k}\|^2-\rho n\|x^{k+1} - x^{k-1}\|^2- \frac{\rho_1}{n}   \left\|\sum_{i=1}^n y_i^{k}\right\|^2
\nonumber\\ \nonumber&- \rho_2 \sum_{i=1}^n  \|y_i^{k}\|^2+\eta L^2 n \|x^k-x^\star\|^2+\frac{1}{\eta} \sum_{i=1}^n \|y_i^k\|^2+\frac{1}{2}\|x^k-x^\star\|^2 + \frac{2 \delta}{n}\sum_{i=1}^{n}\| {u}_i^k-{u}^\star(x^k)\|^2+  \frac{2L^2}{\mu^2}\| x^k-x^{k-1}\|^2\\
&\leq  \frac{1}{\rho} \sum_{i=1}^n \|\lambda_i^{k-1} - \lambda_i^\star\|^2+\rho n\|x^{k}-x^{k-1}\|^2-3\rho n \|y^{k}\|^2-\rho n\|x^{k+1} - x^{k-1}\|^2- \rho_1 n  \| y^{k}\|^2
\nonumber\\&- \rho_2 \sum_{i=1}^n  \|y_i^{k}\|^2+\eta L^2 n \|x^k-x^\star\|^2+\frac{1}{\eta} \sum_{i=1}^n \|y_i^k\|^2 +\frac{1}{2}\|x^k-x^\star\|^2 + \frac{2 \delta}{n}\sum_{i=1}^{n}\| {u}_i^k-{u}^\star(x^k)\|^2+  \frac{2L^2}{\mu^2}\| x^k-x^{k-1}\|^2.
\end{align}
Re-arranging the terms, we obtain
\begin{align}\label{them1inq1}
\nonumber &\frac{1}{\rho} \sum_{i=1}^n \|\lambda_i^k - \lambda_i^\star\|^2  + (\rho+\rho_1) n\|x^{k+1}-x^{k}\|^2+\|x^{k+1} - x^\star\|^2\\
&\leq  \frac{1}{\rho} \sum_{i=1}^n \|\lambda_i^{k-1} - \lambda_i^\star\|^2+\rho n\|x^{k}-x^{k-1}\|^2-3\rho n \|y^{k}\|^2-\rho n\|x^{k+1} - x^{k-1}\|^2- \rho_2 \sum_{i=1}^n  \|y_i^{k}\|^2
\nonumber\\&+\eta L^2 n \|x^k-x^\star\|^2+\frac{1}{\eta} \sum_{i=1}^n \|y_i^k\|^2+\frac{1}{2}\|x^k-x^\star\|^2 + \frac{2 \delta}{n}\sum_{i=1}^{n}\| {u}_i^k-{u}^\star(x^k)\|^2 +  \frac{2L^2}{\mu^2}\| x^k-x^{k-1}\|^2.
\end{align}

%\begin{align}\label{them1inq1}
%\frac{1}{\rho} \sum_{i=1}^N \|\lambda_i^k - \lambda_i^\star\|^2  +\rho N\|x^{k+1}-x^{k}\|^2+\|x^{k+1} - x^\star\|^2+ \rho_1 N  \| x^{k+1}-x^{k}\|^2
%\leq&  \frac{1}{\rho} \sum_{i=1}^N \|\lambda_i^{k-1} - \lambda_i^\star\|^2+\rho N\|x^{k}-x^{k-1}\|^2\nonumber\\
%&-3\rho N \|y^{k}\|^2-\rho N\|x^{k+1} - x^{k-1}\|^2
%\nonumber\\&- \rho_2 \sum_{i=1}^N  \|y_i^{k}\|^2+\eta L^2N \|x^k-x^\star\|^2+\frac{1}{\eta} \sum_{i=1}^N \|y_i^k\|^2\nonumber\\
%&+\frac{1}{2}\|x^k-x^\star\|^2 + \frac{2 \eta}{n}\sum_{i=1}^{N}\| {u}_i^k-{u}^\star(x^k)\|^2\nonumber\\
%&+  2L^2\bigg(\sum_{i=1}^N H_i^0\bigg)^{-2}\| x^k-x^{k-1}\|^2.
%\end{align}

%\begin{align}\label{them1inq1}
%\frac{1}{\rho} \sum_{i=1}^N \|\lambda_i^k - \lambda_i^\star\|^2  +N(\rho+\rho_1) \|x^{k+1}-x^{k}\|^2+\|x^{k+1} - x^\star\|^2+ 
%\leq&  \frac{1}{\rho} \sum_{i=1}^N \|\lambda_i^{k-1} - \lambda_i^\star\|^2+\rho N\|x^{k}-x^{k-1}\|^2\nonumber\\
%&-3\rho N \|y^{k}\|^2-\rho N\|x^{k+1} - x^{k-1}\|^2
%\nonumber\\&- \rho_2 \sum_{i=1}^N  \|y_i^{k}\|^2+\eta L^2N \|x^k-x^\star\|^2+\frac{1}{\eta} \sum_{i=1}^N \|y_i^k\|^2\nonumber\\
%&+\frac{1}{2}\|x^k-x^\star\|^2 + \frac{2 \eta}{n}\sum_{i=1}^{N}\| {u}_i^k-{u}^\star(x^k)\|^2\nonumber\\
%&+  2L^2\bigg(\sum_{i=1}^N H_i^0\bigg)^{-2}\| x^k-x^{k-1}\|^2.
%\end{align}
Choosing $\rho_2 > \frac{1}{\eta}$, we get
\begin{align}\label{them1inq1}
\nonumber &\frac{1}{\rho} \sum_{i=1}^n \|\lambda_i^k - \lambda_i^\star\|^2  + (\rho+\rho_1) n \|x^{k+1}-x^{k}\|^2+\|x^{k+1} - x^\star\|^2\\
\nonumber &\leq  \frac{1}{\rho} \sum_{i=1}^n \|\lambda_i^{k-1} - \lambda_i^\star\|^2+\rho n\|x^{k}-x^{k-1}\|^2 -3\rho n \|y^{k}\|^2-\rho n\|x^{k+1} - x^{k-1}\|^2 +\eta L^2 n \|x^k-x^\star\|^2\\
\nonumber &+\frac{1}{2}\|x^k-x^\star\|^2 + \frac{2 \delta}{n}\sum_{i=1}^{n}\| {u}_i^k-{u}^\star(x^k)\|^2 +  \frac{2L^2}{\mu^2}\| x^k-x^{k-1}\|^2 \\
&\leq  \frac{1}{\rho} \sum_{i=1}^n \|\lambda_i^{k-1} - \lambda_i^\star\|^2+\left(\rho n+\frac{2L^2}{\mu^2}\right)\|x^{k}-x^{k-1}\|^2 +\left(\eta L^2 n+\frac{1}{2}\right) \|x^k-x^\star\|^2\nonumber\\
&+ \frac{2 \delta}{n}\sum_{i=1}^{n}\| {u}_i^k-{u}^\star(x^k)\|^2-3\rho n \|y^{k}\|^2-\rho n\|x^{k+1} - x^{k-1}\|^2.
\end{align}
Choosing $\rho_1=\frac{2L^2}{n \mu^2}$, we get
\begin{align}\label{them1inq1}
&\nonumber\frac{1}{\rho} \sum_{i=1}^n \|\lambda_i^k - \lambda_i^\star\|^2  + n(\rho+\rho_1) \|x^{k+1}-x^{k}\|^2+\|x^{k+1} - x^\star\|^2
\\ &\nonumber \leq \frac{1}{\rho} \sum_{i=1}^n \|\lambda_i^{k-1} - \lambda_i^\star\|^2+ n(\rho+\rho_1)\|x^{k}-x^{k-1}\|^2 + \left(\eta L^2 n+\frac{1}{2}\right) \|x^k-x^\star\|^2+ \frac{2 \delta}{n}\sum_{i=1}^{n}\| {u}_i^k-{u}^\star(x^k)\|^2\nonumber\\
&-3\rho n \|y^{k}\|^2-\rho n\|x^{k+1} - x^{k-1}\|^2.
\end{align}
Choosing $\eta=\frac{1}{2L^2N}$, we get
\begin{align}\label{them1inq1}
\nonumber &\frac{1}{\rho} \sum_{i=1}^n \|\lambda_i^k - \lambda_i^\star\|^2  + n(\rho+\rho_1) \|x^{k+1}-x^{k}\|^2+\|x^{k+1} - x^\star\|^2 \\
&\leq  \frac{1}{\rho} \sum_{i=1}^n \|\lambda_i^{k-1} - \lambda_i^\star\|^2+n(\rho+\rho_1)\|x^{k}-x^{k-1}\|^2+\|x^k-x^\star\|^2 + \frac{2 \delta}{n}\sum_{i=1}^{n}\| {u}_i^k-{u}^\star(x^k)\|^2\nonumber\\
&-3\rho n \|y^{k}\|^2-\rho n\|x^{k+1} - x^{k-1}\|^2.
\end{align}
Next, we define a Lyapunov function $V^k$ as follows
\begin{align}
    V^k = \frac{1}{\rho} \sum_{i=1}^n \|\lambda_i^k - \lambda_i^\star\|^2  + n \left(\rho+\frac{2L^2}{n \mu^2}\right) \|x^{k+1}-x^{k}\|^2+\|x^{k+1} - x^\star\|^2.
\end{align}
Then, we can write
\begin{align}\label{them1inq1}
V^k \leq  V^{k-1}+ \frac{2 \delta}{n}\sum_{i=1}^{n}\| {u}_i^k-{u}^\star(x^k)\|^2-3\rho n \|y^{k}\|^2-\rho n\|x^{k+1} - x^{k-1}\|^2.
\end{align}

From \citep{}, under assumptions that hold for hour dynamic function \textcolor{red}{Amrit, plz check the assumptions}, we have

\begin{align}\label{them1inq1}
\sum_{i=1}^{n}\| {u}_i^k-{u}^\star(x^k)\|^2 \leq \frac{1}{\sqrt{(1+\sigma)}}\sum_{i=1}^{n}\| {u}_i^{k-1}-{u}^\star(x^{k-1})\|^2
\end{align}

\fi
